# Supplementary material for: Non-Autoregressive Neural Machine Translation: A Call for Clarity
Source: arXiv:2205.10577 source file (2022-10-21)
Supplement: Supplementary file 1 [file final_model_stats.tex]

Since we observe very similar translation quality gains for using \ctc with either \glat or \ds, we try to understand how the latter influences the training procedure. In essence, deep supervision, which doesn't include layer-wise prediction-awareness as described in \Cref{sec.ds}, only constraints the decoder to keep a decodeable representation at each layer. Looking into some of the Frobenius norms for the converged model weights in \Cref{fg.enc.norms,fg.dec.norms}, we observe similar trends for \ctc and \ctc + \glat but very different norm layer-trends for \ctc + \ds, especially noticeable in the decoder. We find the encoder norms to be overall fairly similar compared to some of the diverging patterns we observe in the decoder.  

Commonly, in the decoder the norms tend to be overall lower (\eg in the fully-connected layers or the self-attention projections) or exhibit an decreasing trend towards the upper layers (\ie cross-attention or self-attention out and value projections). Unfortunately, simply increasing the weight decay factor doesn't lead to reproducing the patterns observed from \ctc + \ds but rather, as expected, the trends stay consistent to \ctc with an overall lower norm per layer. We also experimented with layer-normalization \citep{ba2016layer} and weight-normalization \citep{SalimansK16}, specifically before the fully-connected layers in the decoder, but couldn't find any immediate way to reproduce the observed behaviour from deep supervision without constraining the representation to be decodeable at each layer.

%%%%%%%%%%%%%%%%%%%%%%%% DECODER %%%%%%%%%%%%%%%%%%%%%%%%%%%%

\begin{figure*}[!htbp]
\begin{subfigure}{\subplotfigsizetriple}
  \centering
  \includegraphics[width=\linewidth]{Figures/Weights/decoder_encoder_attn.k_proj_norm_subplot=True.pdf}  
  \caption{Cross-Attention key $\bm{k}$ Projection}
  \label{fg.dec.cak}
\end{subfigure}
\hfill
\begin{subfigure}{\subplotfigsizetriple}
  \centering
  \includegraphics[width=\linewidth]{Figures/Weights/decoder_encoder_attn.out_proj_norm_subplot=True.pdf}  
  \caption{Cross-Attention out Projection}
  \label{fg.dec.cao}
\end{subfigure}
\hfill
\begin{subfigure}{\subplotfigsizetriple}
  \centering
  \includegraphics[width=\linewidth]{Figures/Weights/decoder_encoder_attn.q_proj_norm_subplot=True.pdf}  
  \caption{Cross-Attention query $\bm{q}$ Projection}
  \label{fg.dec.caq}
\end{subfigure}
\par\bigskip % force a bit of vertical whitespace
\begin{subfigure}{\subplotfigsizetriple}
  \centering
  \includegraphics[width=\linewidth]{Figures/Weights/decoder_encoder_attn.v_proj_norm_subplot=True.pdf}  
  \caption{Cross-Attention value $\bm{v}$ Projection}
  \label{fg.dec.cav}
\end{subfigure}
\hfill
\begin{subfigure}{\subplotfigsizetriple}
  \centering
  \includegraphics[width=\linewidth]{Figures/Weights/decoder_encoder_attn_layer_norm_norm_subplot=True.pdf}  
  \caption{Cross-Attention Layer Norm}
  \label{fg.dec.caln}
\end{subfigure}
\hfill
\begin{subfigure}{\subplotfigsizetriple}
  \centering
  \includegraphics[width=\linewidth]{Figures/Weights/decoder_fc1_norm_subplot=True.pdf}  
  \caption{Fully-connected Layer 1}
  \label{fg.dec.fc1}
\end{subfigure}
\par\bigskip % force a bit of vertical whitespace
\begin{subfigure}{\subplotfigsizetriple}
  \centering
  \includegraphics[width=\linewidth]{Figures/Weights/decoder_fc2_norm_subplot=True.pdf}  
  \caption{Fully-connected Layer 2}
  \label{fg.dec.fc2}
\end{subfigure}
\hfill
\begin{subfigure}{\subplotfigsizetriple}
  \centering
  \includegraphics[width=\linewidth]{Figures/Weights/decoder_final_layer_norm_norm_subplot=True.pdf}  
  \caption{Final Layer Norm}
  \label{fg.dec.final_ln}
\end{subfigure}
\hfill
\begin{subfigure}{\subplotfigsizetriple}
  \centering
  \includegraphics[width=\linewidth]{Figures/Weights/decoder_self_attn.k_proj_norm_subplot=True.pdf}  
  \caption{Self-Attention key $\bm{k}$ Projection}
  \label{fg.dec.sak}
\end{subfigure}
\par\bigskip % force a bit of vertical whitespace
\begin{subfigure}{\subplotfigsizetriple}
  \centering
  \includegraphics[width=\linewidth]{Figures/Weights/decoder_self_attn.out_proj_norm_subplot=True.pdf}  
  \caption{Self-Attention out Projection}
  \label{fg.dec.sao}
\end{subfigure}
\hfill
\begin{subfigure}{\subplotfigsizetriple}
  \centering
  \includegraphics[width=\linewidth]{Figures/Weights/decoder_self_attn.q_proj_norm_subplot=True.pdf}  
  \caption{Self-Attention query $\bm{q}$ Projection}
  \label{fg.dec.saq}
\end{subfigure}
\hfill
\begin{subfigure}{\subplotfigsizetriple}
  \centering
  \includegraphics[width=\linewidth]{Figures/Weights/decoder_self_attn.v_proj_norm_subplot=True.pdf}  
  \caption{Self-Attention value $\bm{v}$ Projection}
  \label{fg.dec.sav}
\end{subfigure}
\par\bigskip % force a bit of vertical whitespace
\begin{subfigure}{\subplotfigsizetriple}
  \centering
  \includegraphics[width=\linewidth]{Figures/Weights/decoder_self_attn_layer_norm_norm_subplot=True.pdf}  
  \caption{Self-Attention Layer Norm}
  \label{fg.dec.saln}
\end{subfigure}
\caption{Frobenius norm of the final decoder component weights across layers. Here displayed are sample runs for \ctc (\squarectc, \emph{valid}: $25.2$, \emph{test}: $25.7$), \ctc with a weight decay of $0.02$ (\squarectcwdpone, \emph{valid}: $24.9$, \emph{test}: $25.4$), \ctc + \ds (\squarectcds, \emph{valid}: $25.4$, \emph{test}: $25.9$), and \ctc + \glat (\squarectcglat, \emph{valid}: $25.5$, \emph{test}: $25.9$) all trained on WMT'14 \lende distilled data. }
\label{fg.dec.norms}
\end{figure*}

%%%%%%%%%%%%%%%%%%%%%%%% ENCODER %%%%%%%%%%%%%%%%%%%%%%%%%%%%

\begin{figure*}[!htbp]
\begin{subfigure}{\subplotfigsizedouble}
  \centering
  \includegraphics[width=\linewidth]{Figures/Weights/encoder_fc1_norm_subplot=True.pdf}  
  \caption{Fully-connected Layer 1}
  \label{fg.enc.fc1}
\end{subfigure}
\hfill
\begin{subfigure}{\subplotfigsizedouble}
  \centering
  \includegraphics[width=\linewidth]{Figures/Weights/encoder_fc2_norm_subplot=True.pdf}  
  \caption{Fully-connected Layer 2}
  \label{fg.enc.fc2}
\end{subfigure}
\par\bigskip % force a bit of vertical whitespace
\begin{subfigure}{\subplotfigsizedouble}
  \centering
  \includegraphics[width=\linewidth]{Figures/Weights/encoder_final_layer_norm_norm_subplot=True.pdf}  
  \caption{Final Layer Norm}
  \label{fg.enc.final_ln}
\end{subfigure}
\hfill
\begin{subfigure}{\subplotfigsizedouble}
  \centering
  \includegraphics[width=\linewidth]{Figures/Weights/encoder_self_attn.k_proj_norm_subplot=True.pdf}  
  \caption{Self-Attention key $\bm{k}$ Projection}
  \label{fg.enc.sak}
\end{subfigure}
\par\bigskip % force a bit of vertical whitespace
\begin{subfigure}{\subplotfigsizedouble}
  \centering
  \includegraphics[width=\linewidth]{Figures/Weights/encoder_self_attn.out_proj_norm_subplot=True.pdf}  
  \caption{Self-Attention out Projection}
  \label{fg.enc.sao}
\end{subfigure}
\hfill
\begin{subfigure}{\subplotfigsizedouble}
  \centering
  \includegraphics[width=\linewidth]{Figures/Weights/encoder_self_attn.q_proj_norm_subplot=True.pdf}  
  \caption{Self-Attention query $\bm{q}$ Projection}
  \label{fg.enc.saq}
\end{subfigure}
\par\bigskip % force a bit of vertical whitespace
\begin{subfigure}{\subplotfigsizedouble}
  \centering
  \includegraphics[width=\linewidth]{Figures/Weights/encoder_self_attn.v_proj_norm_subplot=True.pdf}  
  \caption{Self-Attention value $\bm{v}$ Projection}
  \label{fg.enc.sav}
\end{subfigure}
\hfill
\begin{subfigure}{\subplotfigsizedouble}
  \centering
  \includegraphics[width=\linewidth]{Figures/Weights/encoder_self_attn_layer_norm_norm_subplot=True.pdf}  
  \caption{Self-Attention Layer Norm}
  \label{fg.enc.saln}
\end{subfigure}
\caption{Frobenius norm of the final encoder component weights across layers. Here displayed are sample runs for \ctc (\squarectc, \emph{valid}: $25.2$, \emph{test}: $25.7$), \ctc with a weight decay of $0.02$ (\squarectcwdpone, \emph{valid}: $24.9$, \emph{test}: $25.4$), \ctc + \ds (\squarectcds, \emph{valid}: $25.4$, \emph{test}: $25.9$), and \ctc + \glat (\squarectcglat, \emph{valid}: $25.5$, \emph{test}: $25.9$) all trained on WMT'14 \lende distilled data. }
\label{fg.enc.norms}
\end{figure*}
