# Supplementary material for: Non-Autoregressive Neural Machine Translation: A Call for Clarity
Source: arXiv:2205.10577 source file (2022-10-21)
Supplement: Supplementary file 2 [file decoder_components.tex]

% \begin{table}[t]
% \centering
% \small
% \tabcolsep 4pt
% \begin{tabular}{lcc}
% \toprule
% \multirow{2}{*}{\textbf{Models}} & \textbf{WMT'13} & \textbf{WMT'14} \\
%  & \textbf{\lende} & \textbf{\lende} \\
% \midrule
%  \textbf{\ctc} & \multirow{2}{*}{24.9} & \multirow{2}{*}{25.8} \\ % gwhcs3rqx6
%  \citep{saharia-etal-2020-non} & & \\[0.1cm]
%   \quad\quad + no layer 0 self attention & 25.0 \chu{0.1} & 25.5 \chd{0.3} \\ % 4dskjp5ydx
%  \quad\quad + no decoder embeddings & 24.7 \chd{0.2} & 25.8 \chd{0.2} \\ % 
%  \quad\quad + both & 24.9 \che{0.0} & 25.5 \chd{0.3} \\ % rvg6ny2cxq
%  \midrule
%  \textbf{\ctc + \glat} & \multirow{2}{*}{25.8} & \multirow{2}{*}{26.0} \\  % xzuk4stdwn
%  \citep{qian-etal-2021-glancing} & & \\[0.1cm] 
%  \quad\quad + no layer 0 self attention & 25.8 \che{0.0} & 25.9 \chd{0.1} \\ % 
%  \bottomrule
% \end{tabular}
% \caption{Overview of the quality implications when removing decoder components. Distilled training data and hyperparameters stay consistent and results are reported for the evaluation sets of WMT'13 and '14 for \lende.}
% \label{tb.decoder_components}
% \end{table}

% In the absence of guided decoder input, one can question the usefulness of a few early decoder components such as the self-attention in the first decoder layer or the decoder embeddings, since only consecutive special tokens \ie \texttt{<unk>}'s are passed and these most likely don't contain much meaningful information. From our experiments for these components when using \ctc and \ctc + \glat, summarized in \Cref{tb.decoder_components}, we conclude that we can safely remove the self-attention in the first decoder layer and the decoder embeddings, as it does not have a big effect on \bleu.
